# Supplementary material for: LSM: Learning Subspace Minimization for Low-level Vision
Source: arXiv:2004.09197 source file (2020-04-20)
Supplement: Supplementary file 1 [file appendix.tex]

\section{Network Structures}
\label{app:net}
\paragraph{Feature Pyramid}
The feature pyramid learns to extract feature maps that measures the channel consistency for objective function and serve as the image context features for subspace prediction. We use DRN-22~\cite{DRN} as the backbone network for efficiency and denote the last residual blocks of conv3, conv4, conv5, conv6 in DRN-22 as $\{C^4,C^3,C^2,C^1\}$, with strides $\{4,8,16,32\}$ respectively. We upsample a feature map $C^{k}$ by a factor of 2 with bilinear interpolation and concatenate the upsampled feature map with $C^{k+1}$ in the next level. This procedure is iterated until the finest level. Finally, we apply a $3\times3$ convolution on the concatenated feature maps to reduce its dimensionality to 128 to balance the expressiveness and computational complexity, which leads to the final feature pyramid $\sF=\{F^{1},F^2,F^3,F^{4},F^{5}\}$.
\paragraph{Subspace Predictor}
The subspace predictor is learned to predicted the basis $\mathcal{V}$ from the image context and the minimization context features. Before feeding the features to the subspace predictor, we average pool the context features with different kernel size to aggregate the spatial information at different scale. Instead of first average pooling with stride and upsampling as in spatial pyramid pooling~\cite{PSPNET,SPP}, we first compute the integral image of each features channel and calculate the pooled features for each pixel coordinate based on the integral image, which gives better efficiency as in computer vision literature~\cite{HARR,GF}. We illustrate the subspace predictor at the finest level in~\figref{SL}, and this design of the subspace predictor is simple yet effective as demonstrated in the experiments and can serve as the baseline for future works. Please refer to the \emph{appendix} for more details.
